# Supplementary material for: Enhanced Modeling of Contingency Response in Security-constrained Optimal Power Flow
Source: arXiv:2102.08579 source file (2021-02-17)
Supplement: Supplementary file 1 [file appendix.tex]

\appendix
The inverters' parameters in the IEEE34-bus system are provided in~\tabref{tab_ieee}.

\begin{table}[h]
\centering
\caption{System Specifications}
\begin{tabular}{l|l|l|l}
VCVSIs& \multicolumn{2}{c|}{Inverters 1 \& 2} & {Inverters 3 \& 4} \\
\hline
\hline
\multirow{2}{*}{Droop} & $m_p$ & $9.4 \times 10^{-5}$  & $12.5 \times 10^{-5}$ \\
 & $n_Q$ & $1.3 \times 10^{-3}$  & $1.5 \times 10^{-5}$\\
\hline
\multirow{2}{*}{Coupling inductance}& $R_c$ & 0.03 $\Omega$ & 0.03 $\Omega$ \\
& $L_c$ & 0.35 mH  & 0.35 mH  \\
\hline
\multirow{3}{*}{LC filter}& $R_f$ & 0.1 $\Omega$ &  0.1 $\Omega$\\
& $L_f$ & 100 $\mu$H & 100 $\mu$H \\
& $C_f$ & 0.7 mF &  0.7 mF \\
\hline
\multirow{4}{*}{Local controller}& $K_{PV}$ & 0.1  & 0.05  \\
& $K_{IV}$ & 420  & 390  \\
& $K_{PC}$ & 15  & 10.5  \\
& $K_{IC}$ & 20000  & 16000  \\ 
\hline
Switching frequency & $f_{sw}$ & 2500 Hz & 2500 Hz \\
\hline 
Input Voltage & $V_{dc}$ & 1000 V & 1000 V \\
\hline
\end{tabular}
\tablabel{tab_ieee}
\end{table}
%

%$,
%\ \mathds{A} = 25 \left[\begin{IEEEeqnarraybox*}[][c]{,c/c,} 0&1\\
%1&0%
%\end{IEEEeqnarraybox*} \right],
%\ \mathds{B}=\mathds{A},
%\mathds{C}=0.5\mathds{A}, 
%I = 3 \left[\begin{IEEEeqnarraybox*}[][c]{,c/c,} 1&0\\
%0&1%
%\end{IEEEeqnarraybox*} \right], P= 0.05\left[\begin{IEEEeqnarraybox*}[][c]{,c/c,} 1&0\\
%0&1%
%\end{IEEEeqnarraybox*} \right], K= \left[\begin{IEEEeqnarraybox*}[][c]{,c/c,} 1&0\\
%0&2%
%\end{IEEEeqnarraybox*} \right]$.
